# Supplementary material for: HighDist Framework: Algorithms and Applications
Source: arXiv:2103.09033 source file (2022-02-22)
Supplement: Supplementary file 1 [file appendix-hd-lowerbound.tex]

\section{Proof of Lemma~\ref{lemma:highdist-lb} (lower bound for \prob)}
\label{sec:highdist-lb}

We first prove that \promiseprob requires $\Omega(\tfrac{1}{\epsilon})$ queries. For this we reduce an instance of \countdec on a $n$-bit string $X$ with $l_1=\tfrac{n}{2}$ and $l_2=\tfrac{n}{2}+\varepsilon n$ to \promiseprob. Observe that an oracle to $X$ can be used to implement an oracle $O_D$ to the distribution $\D$ induced by the frequencies of 0 and 1 in $X$, and each call to $O_D$ corresponds to one call to $X$ (see Section~\ref{subsec:oracle}). By Theorem~\ref{thm:nayak_wu}, the query complexity to decide the above \countdec instance is $\Omega(\tfrac{n}{\varepsilon n/2})$. If $|X|=\tfrac{n}{2}$ then $\Pr_D[0]=\Pr_D[1]=\tfrac{1}{2}$, and if $|X|=\tfrac{n}{2}+\varepsilon n$, then $\Pr_D[1]=\tfrac{1}{2}+\varepsilon$. Thus, the output of a \promiseprob algorithm with $\tau=\tfrac{1}{2}+\varepsilon$ and additive accuracy $\epsilon=\varepsilon$ can be used to decide our \countdec instance. This proves a lower bound of $\Omega(\tfrac{1}{\varepsilon})=\Omega(\tfrac{1}{\epsilon})$ for \promiseprob, and also of its generalized version \prob.

Next we prove another bound of $\Omega(\tfrac{1}{\sqrt{\tau}})$. Together they prove Lemma~\ref{lemma:highdist-lb}.

For proving this lower bound, instead of the \countdec problem, we use the quantum adversary method. We first use this method to obtain a lower bound on the mode decision problem: Given an array $A$ of size $n$ and a threshold $\tau'\in[1,n]$ we have to decide if there exists any element whose frequency is greater than $\tau'$.
We then show a reduction from mode decision problem to \prob to get a lower bound on it.

The main theorem of quantum adversary method can be stated as below~\cite{adversarymethod}:
\begin{theorem}
\label{thm:qa_method}
Let $F$ be a $n$-bit Boolean function and $X$ and $Y$ be two sets of inputs such that $F(x)\neq F(y)$ for any $x\in X$ and $y\in Y$. Let $R\subseteq X\times Y$ be a relation such that 
\begin{enumerate}
    \item for every $x \in X$, $\exists$ at least $m$ different $y \in Y$ such that $(x,y)\in R$.
    \item for every $y \in Y$, $\exists$ at least $ m'$ different $x \in X$ such that $(x,y)\in R$.
    \item for every $x \in X$ and $i \in \{1,...,n\}$, $\exists$ at most $l$ different $y \in Y$ such that $x_i \neq y_i$ and $(x,y)\in R$.
    \item for every $y \in Y$ and $i \in \{1,...,n\}$, $\exists$ at most $l'$ different $x \in X$ such that $x_i \neq y_i$ and $(x,y)\in R$.
\end{enumerate}
Then any quantum algorithm uses $\Omega\Big(\sqrt{\frac{m\cdot m'}{l\cdot l'}}\Big)$ queries to compute $F$ on $X \bigcup Y$.
\end{theorem}

Consider the mode decision problem.  
Let $\tau'\in [1,n]$ be a threshold and set $t = \frac{n}{\tau'-1}$. 
Let $F$ be a Boolean function such that $F(x)=1$ if $x$ is an array whose modal value is greater than or equal to $\tau'$ and $F(y)=0$ if the modal value of $y$ is strictly less than $\tau'$.
Let $X$ be the set of all arrays $A$ of size $n$ such that there is exactly one element with frequency $\tau'$, one element with frequency $(\tau'-2)$ and all other elements with frequency $(\tau'-1)$.
Let $a_1$ be the mode of array $A$ and the other elements be $a_2, a_3, \cdots, a_t$.
Also, let $Y$ be the set of all arrays $B$ of size $n$ such that all the elements of $B$ occur with frequency $(\tau'-1)$.
It is easy to see that the number of unique elements is $t$.
Define a relation $R$ such that a tuple of arrays $(A,B)$ belong to $R$ if and only if $A$ and $B$ match at all but $1$ indices and the mode of $A$ is the first element of $B$, say $b^{(1)}$.

Now, for any $A\in X$, construct $A_{i,\tilde{a}}'$ for $i\in [n]$ and $\tilde{a}\in \{a_2, a_3, \cdots, a_n\}$ such that (i) if $A[i]\neq a_1$, then $A_{i,\tilde{a}}' = A$, else (ii) $A_{i,\tilde{a}}'[k] = A[k]$ when $k\neq i$ and $A_{i,\tilde{a}}'[i] = \tilde{a}$.
Then, for $A$, there exists exactly $\tau'(t-1)$ many $A_{i, \tilde{a}}'$ arrays such that they belong to $Y$.
Notice that any $\Aitil$ of an array $A\in X$ such that $A[i]=a_1$ also satisfy $(A, \Aitil)\in R$.

For any $A\in X$ and $i\in [n]$, it is immediate that there are at most $(t-1)$ many $\tilde{a}$'s such that $A[i]\neq \Aitil[i]$ and $(A, \Aitil)\in R$ since $\Aitil$ has to be equal to $A$ at all indices except $i$ and at $i$, $\Aitil$ can take one of the values from $\{a_2, a_3, \cdots a_t\}$.

Next, for any $B\in Y$, construct $B_i'$ such that $B_i' = B$ (i) if $B[i]=b^{(1)}$ then $B_i'=B$, else (ii) $B_i'[k]=B[k]$ for $k\neq i$ and $B_i'[i] = b^{(1)}$.
Then, for $B$, there exists exactly $n-\tau'+1$ many $i$'s such that $B_i'\in X$ and $(B_i', B)\in R$.

Also, for any $B\in Y$ and $i\in [n]$, there is at most one $B_i'$ such that $B_i'[i]\neq B[i]$ and $(B_i', B)\in R$.

From these constructions, we can derive that the quantum query complexity of computing $F$ is $\Omega\Big(\sqrt{\frac{\tau'(t-1)\cdot (n-\tau'+1)}{(t-1)\cdot 1}}\Big) = \Omega\big(\sqrt{\tau'(n-\tau')}\big)$ queries.

Now, the reduction from the mode decision problem to \prob can be trivially done by setting the threshold of \prob $\tau$ as $\tau = \tau'/n$ and the additive accuracy of \prob $\epsilon$ as $\epsilon = \epsilon'/n$.
This would imply that the quantum query lower bound of \prob is $\Omega(n\sqrt{\tau(1-\tau')})$ for $\epsilon=\frac{1}{n}$.
